# Supplementary material for: Investigating the Requirements for Building a Blockchain Simulator for IoT Applications
Source: arXiv:2208.11207 source file (2022-08-23)
Supplement: Supplementary file 1 [file Questionnaire_pdf.pdf]

## An Efficient Simulation Framework for Modelling the Behaviour of Blockchain based IoT ecosystems

This survey is part of a Ph.D. research project titled: ‘An Efficient Simulation Framework for Modelling the Behaviour of Blockchain based IoT ecosystems’. This work is conducted by Adel Mohammed Albshri, a researcher from Newcastle University - the United Kingdom.

Blockchain is a technology that facilitates distributed, transparent, and secure data sharing and storage, features which we believe can be used as a base for enhancing secure IoT applications. We are pleased to invite you to participate in this study, which aims to determine the requirements and sets of features that are needed as part of a Blockchain based Internet of Things simulation environment. This survey is designed mainly to gather the opinions of IoT and/or blockchain engineers and practitioners.

A set of questions about the IoT blockchain simulator we propose will be presented. We anticipate that it will take no more than 5–10 minutes to complete the questionnaire.

The University of Newcastle’s Ethics Committee has given approval for the project. All information gathered during this research will be kept secure and anonymous. A password-protected laptop will be used to store the data, and only the primary researcher will have access to it. Further, each participant will be randomly assigned a number (P1, P2, etc), to protect the data and organise it prior to analysis.

If you have any questions regarding this research, you are welcome to contact me at any time using the email address A.Albshri2@ncl.ac.uk

* 1. Do you agree to participate in this survey?

☐ I agree to participate in this survey.

This data will remain anonymous and will not be released to the public and it is only used within this research for the purpose of further communication.

2. Name (optional)

3. Email (optional)

## An Efficient Simulation Framework for Modelling the Behaviour of Blockchain based IoT ecosystems

Please indicate your basic preference level, from low to high, for the questions below using the following scale.

The Internet of Things (IoT) is a distributed eco-system that consists of objects/entities that communicate over a computer network, such as the public Internet.

* 4. To what extent you are familiar with IoT?

| Low | Moderately low | Moderately | Moderately high | High |
|---|---|---|---|---|
| ○ | ○ | ○ | ○ | ○ |

Blockchain uses a distributed/shared database that logs all executed transactions in a network while providing a wide range of properties, such as trust, transparency, and immutability.

* 5. To what extent you are familiar with blockchain?

| Low | Moderately low | Moderately | Moderately high | High |
|---|---|---|---|---|
| ○ | ○ | ○ | ○ | ○ |

**An Efficient Simulation Framework for Modelling the Behaviour of Blockchain based IoT ecosystems**

Please indicate, using the scale provided, to what extent you agree or disagree with the following statements.

Blockchain with a decentralized core is liable for guaranteeing high data security levels, as it is a tamper-proof technology. At the same time, IoT is a distributed system wherein data can be stored in multiple components such, as edge devices. In other words, IoT is the technology paving roads for a digital smart world.

*6- From my perspective, there may be an expansion of blockchain technology along with the Internet of things (IoT) in the future.

| Strongly agree | Agree | Neutral | Disagree | Strongly disagree |
|---|---|---|---|---|
| ○ | ○ | ○ | ○ | ○ |

Naturally, as the configuration settings (e.g., block size, # of miner nodes, # of transactions per block, etc.) vary, the system's performance (e.g., scalability, security, etc.) is greatly affected.

* 7. Do you think that there is a need for an IoT blockchain simulator that helps developers to systematically adjust the system's configurations?

| Strongly agree | Agree | Neutral | Disagree | Strongly disagree |
|---|---|---|---|---|
| ○ | ○ | ○ | ○ | ○ |

IoT devices consist of sensors, actuators, and mobile devices that can sense the physical environment and transfer data to edge or cloud data centers for further analysis. For example, personal monitoring devices (like wearable watches) sense the physical state of the patient and transmit their data to hospital tracking systems. Then, physicians (or a smart diagnosis system) diagnosis the case in real-time.

* 8. Do you agree that all IoT data should be stored in the blockchain?

| Strongly agree | Agree | Neutral | Disagree | Strongly disagree |
|---|---|---|---|---|
| ○ | ○ | ○ | ○ | ○ |

Consensus algorithms are liable for choosing a miner node to fabricate the blocks. The strategy used to pick miners' changes differs among blockchains and is contingent upon the received consensus algorithms

* 9. Do you prefer having an IoT blockchain simulator that makes use of different types of consensus algorithms?

| Strongly agree | Agree | Neutral | Disagree | Strongly disagree |
|---|---|---|---|---|
| ○ | ○ | ○ | ○ | ○ |

To gain insight into the latency of transactions, it is of great importance that we have the ability to access the full log information of those transactions.

10. Do you prefer having the flexibility to investigate the detailed log information for every transaction?

| Strongly agree | Agree | Neutral | Disagree | Strongly disagree |
|---|---|---|---|---|
| ◯ | ◯ | ◯ | ◯ | ◯ |

Nodes are the essential component of blockchain infrastructure. In the blockchain, nodes are connected, and they constantly exchange the latest blockchain data with each other; this protocol keeps nodes updated. In the context of IoT, data from the IoT devices are processed closer to where they are generated via edge devices such as Raspberry Pi, rather than sent over long routes to data centers or the cloud.

* 11. Do you agree with using IoT edge devices like Raspberry Pi (RPi) as the blockchain nodes?

| Strongly agree | Agree | Neutral | Disagree | Strongly disagree |
|---|---|---|---|---|
| ◯ | ◯ | ◯ | ◯ | ◯ |

Blockchain has different types, like public and private. A “one type fits all application” policy may lead to a high degree of performance degradation.

* 12. Would you prefer to have a simulator capable of modelling every type of blockchain?

| Strongly agree | Agree | Neutral | Disagree | Strongly disagree |
|---|---|---|---|---|
| ◯ | ◯ | ◯ | ◯ | ◯ |
